# Supplementary material for: Backaction suppression in levitated optomechanics using reflective boundaries
Source: arXiv:2405.04366 source file (2025-04-25)
Supplement: Supplementary file 1 [file supplementary.tex]

% ****** Start of file apstemplate.tex ****** %
%%
%%
%%   This file is part of the APS files in the REVTeX 4.2 distribution.
%%   Version 4.2a of REVTeX, January, 2015
%%
%%
%%   Copyright (c) 2015 The American Physical Society.
%%
%%   See the REVTeX 4 README file for restrictions and more information.
%%
%
% This is a template for producing manuscripts for use with REVTEX 4.2
% Copy this file to another name and then work on that file.
% That way, you always have this original template file to use.
%
% Group addresses by affiliation; use superscriptaddress for long
% author lists, or if there are many overlapping affiliations.
% For Phys. Rev. appearance, change preprint to twocolumn.
% Choose pra, prb, prc, prd, pre, prl, prstab, prstper, or rmp for journal
%  Add 'draft' option to mark overfull boxes with black boxes
%  Add 'showkeys' option to make keywords appear

%\documentclass[aps,prl,preprint,groupedaddress]{revtex4-2}  % SHOULD PROBABLY USE THIS

%\documentclass[aps,prl,preprint,superscriptaddress]{revtex4-2}
\documentclass[reprint,groupedaddress]{revtex4-2}

\usepackage{graphicx}
\usepackage{upgreek}
\usepackage{amsmath, amssymb}
\usepackage{lipsum}
\usepackage{stackengine}

\usepackage{color} % for the command \textcolor
\usepackage{soul} % for the command \hl
\usepackage{hyperref}
\hypersetup{
    colorlinks=true,
    linkcolor=blue,
    filecolor=magenta,      
    citecolor=blue,      
    urlcolor=blue,
    }
\urlstyle{same}

\DeclareMathAlphabet\mathbfcal{OMS}{cmsy}{b}{n}

% units in equations

% symbols

% enclosing environments

% unit vectors

% fluctuations

% frequency

% dyadics

% useful shortcuts

% \input{newcommands}
\begin{document}
\title{Supplementary material: Backaction suppression in levitated optomechanics}

\author{Rafa{\l} Gajewski}
\author{James Bateman}
\email[]{j.e.bateman@swansea.ac.uk}
\affiliation{Department of Physics, Faculty of Science and Engineering, Swansea University, SA2 8PP UK}

\date{\today}
\maketitle
\onecolumngrid
\input{farfields_supplement}
\input{backaction_supplement}
\bibliography{main}
\end{document}
